# Supplementary material for: Run Your Visual-Inertial Odometry on NVIDIA Jetson: Benchmark Tests on a Micro Aerial Vehicle
Source: arXiv:2103.01655 source file (2021-03-02)
Supplement: Supplementary file 1 [file 6.appendix.tex]

\section*{APPENDIX}

% 깃랩링크
